# Supplementary material for: In-Hand 3D Object Scanning from an RGB Sequence
Source: arXiv:2211.16193 source file (2023-06-22)

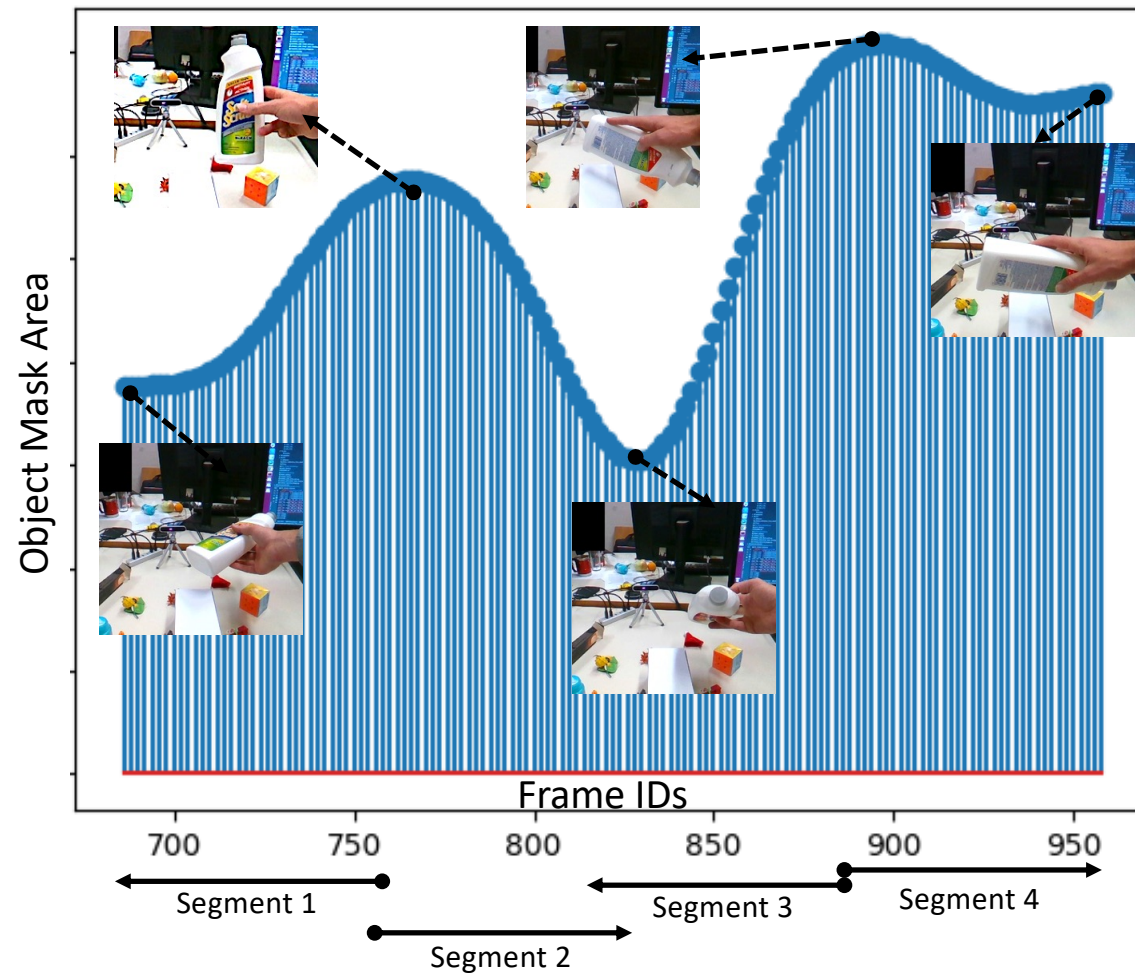

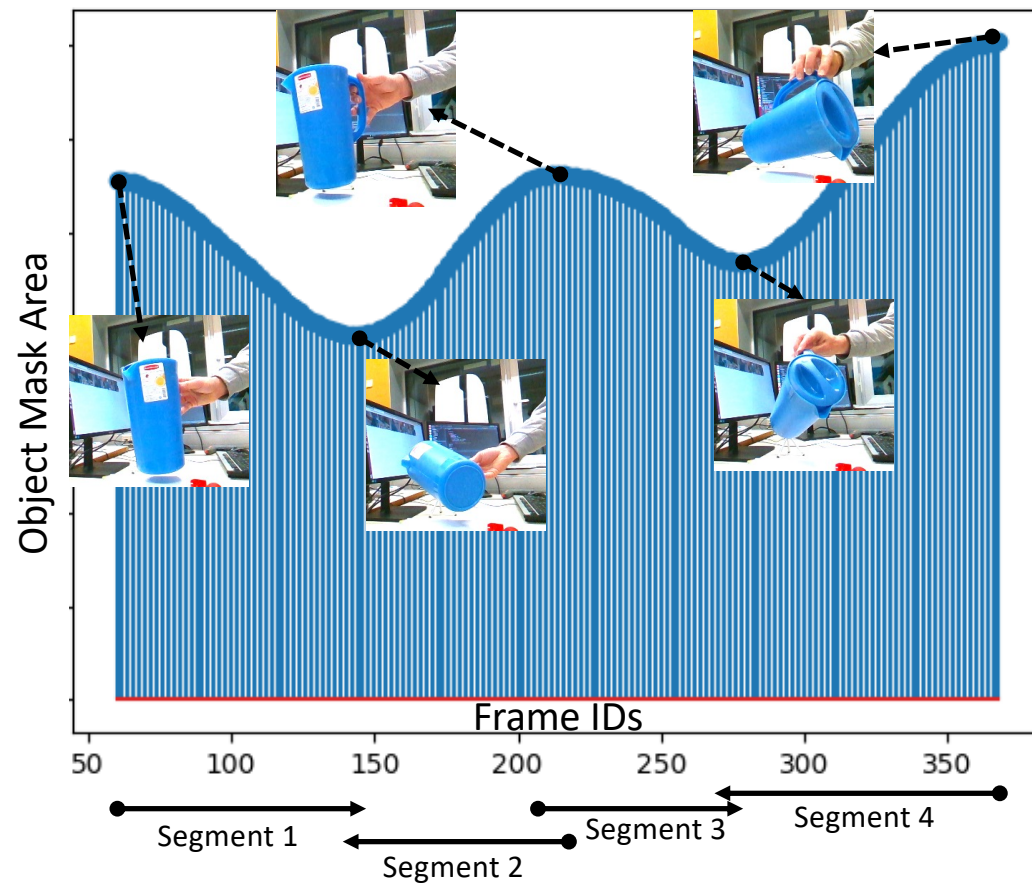

Supplement: Supplementary file 2 [file area_curves.pdf]
